# Supplementary material for: Compass-V2 Technical Report
Source: arXiv:2504.15527 source file (2025-04-22)
Supplement: Supplementary file 1 [file 10_appendix.tex]

\section{Appendix} \label{appendix}

\subsection{Compass Portal Introduction}

Compass Portal is a web-based conversational interface similar to ChatGPT, enabling users to rapidly explore the multifaceted capabilities of the Compass series of large language models. These capabilities include, but are not limited to, deep reasoning and web-based information retrieval.

\begin{figure}[htbp]
    \centering
    \includegraphics[width=0.85\textwidth]{./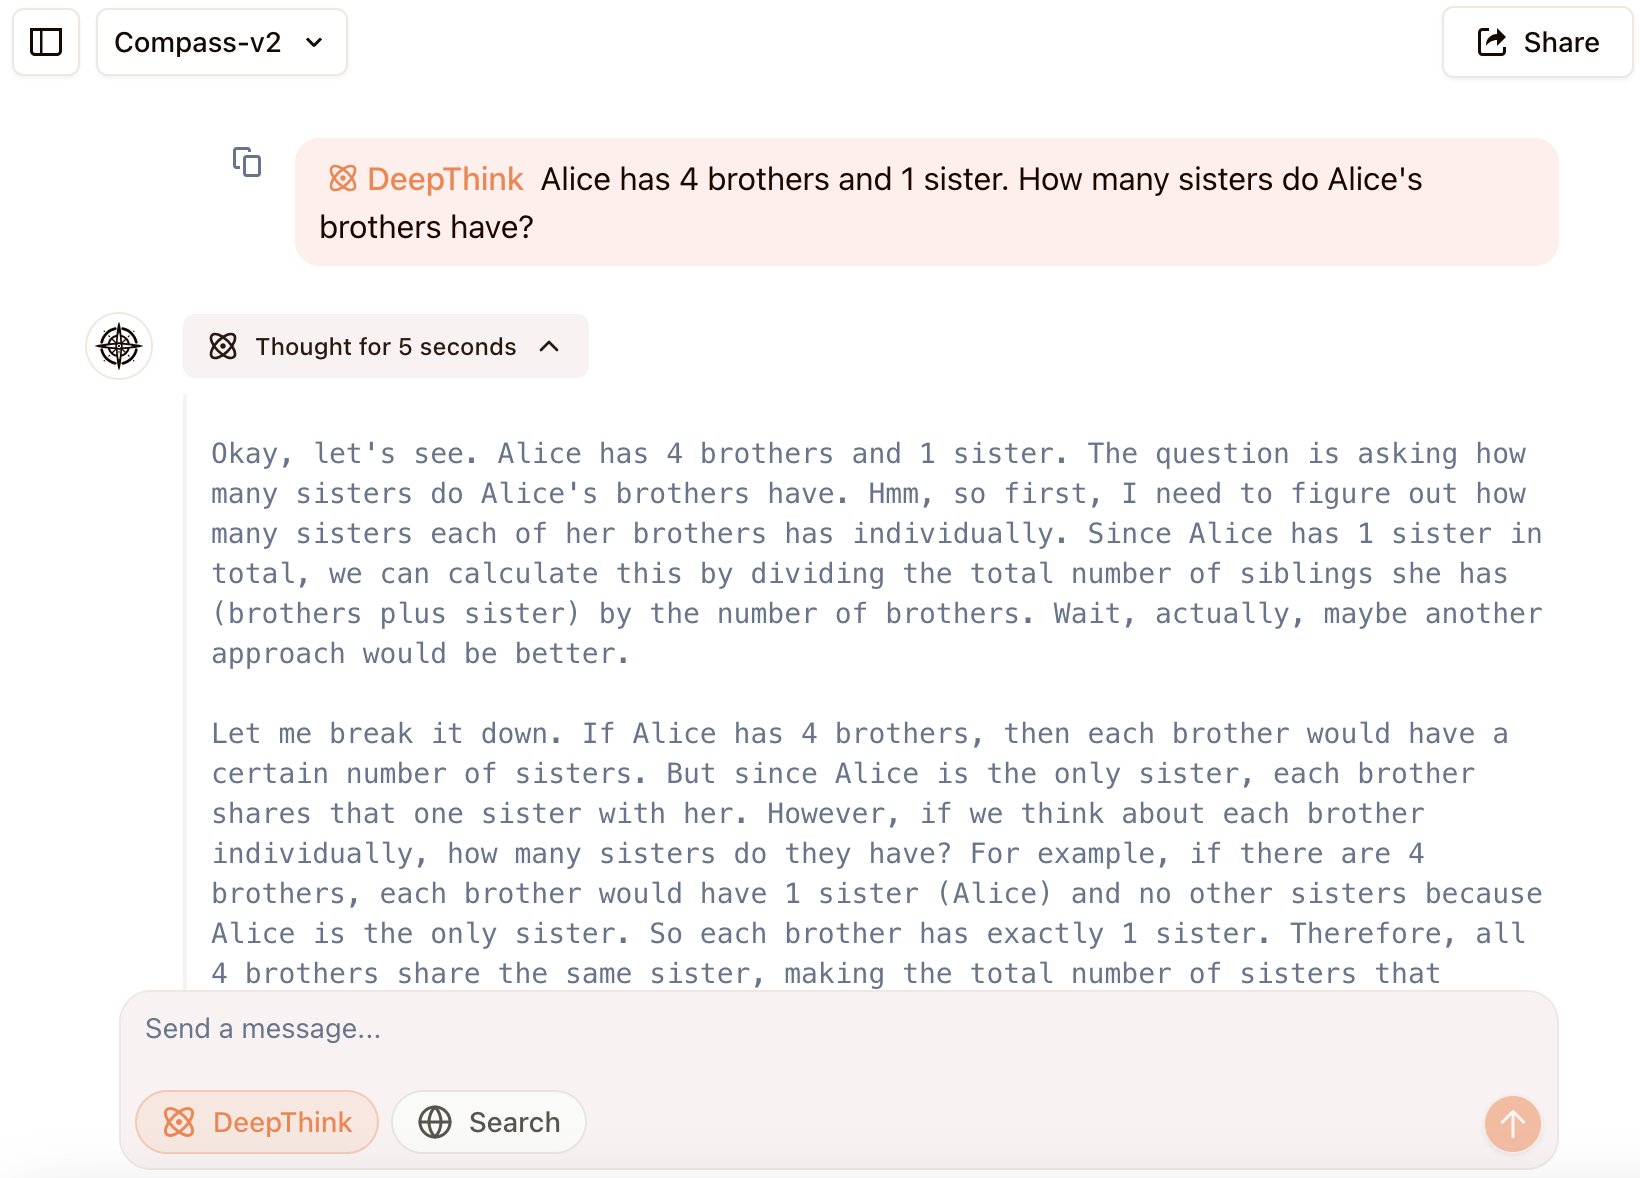}
    \caption{Demo of Compass-v2}
    \label{fig:demo}
\end{figure}

\subsection{Roleplay Prompt Design}
\begin{table}[h!]
\caption{Prompts for role-playing dataset construction}
    \centering
    \begin{tabular}{p{12cm}}
    \toprule
    \textbf{System Prompt for Role-playing} \\
    \hline
    I want you to act like \{character\}. I want you to respond and answer using the tone, manner and vocabulary that would be appropriate, using all relevant knowledge for this \{character\} in English/Chinese. \\
    % \vspace{1em}
    Character Name: \\
    \{character\} (Necessary) \\
    % \vspace{1em}
    The context is as follows: \\
    \{context\} (if available) \\
    % \vspace{1em}
    The profile of \{character\} is as follows: \\
    \{character\_profile\} (if available) \\
    % \vspace{1em}
    Here is your knowledge about the other characters: \\
    \{other\_character\_profiles\_str\} (if available) \\
    % \vspace{1em}
    Other restrictions: \\
    \{other\_restrictions\} (if available) \\
    % \vspace{1em}
    The Current Scenario is as follows: \\
    Location: \\ \{location\} (if available) \\
    Status: \\ \{Status\} (if available) \\
    \bottomrule
    \end{tabular}
    
    \label{tab:roleplay_prompt_design}
\end{table}

\subsection{LongCoT Responses Cases} \label{appendix:longcot}
Below is the LongCot response case from Compass-v2.
\begin{table}[hbp]
    \caption{Responses cases comparison}
    \begin{tcolorbox}[title=LongCoT, colframe=red!50!black, colback=red!5!white]
    \textbf{<System>:} Let's think step by step. Please ensure that the reasoning process are enclosed within <think> </think> tags, i.e., <think> reasoning process here </think>. And put your final answer within \verb|\boxed{}|.
    
    \textbf{<Human>:} How many r in word strawberry?
    \tcblower
    
    \textbf{<AI>:} <think>
    Okay, let's see. The question is asking how many 'r's are in the word "strawberry." Hmm, I need to break this down step by step. First, I should make sure I spell the word correctly in my mind. "Strawberry," right? Not "strawberrye" or something else. Yeah, that's the correct spelling.

    Now, to count the number of 'r's, I'll go through each letter one by one. Let's start from the beginning: S-T-R-A-W. So the first letter is 'S', not an 'r'. Then the second letter is 'T'. Third is 'R'. Okay, here we go, the first 'r' is at the third position. 
    
    Continuing, the fourth letter is 'A', fifth is 'W', sixth is 'A', seventh is 'Y'. Wait, hold on. Let me check again. Let's write out the word slowly: S-T-R-A-W-A-R-R-Y. Wait, is that right? Let me count the letters. S (1), T (2), R (3), A (4), W (5), A (6), R (7), R (8), Y (9). Yes, so there are nine letters in total. Now, the 'r's are at positions 3, 7, and 8. That makes three 'r's. 
    
    But wait, sometimes people might miss one if they rush. Let me verify again. Starting from the beginning: S, T, R, A, W, A, R, R, Y. Yep, the 'R's are the third, seventh, and eighth letters. So three 'r's in total. I think that's correct. I don't recall any other 'r's in the word. Let me confirm with another method. If I say the word aloud, emphasizing each sound: "straw-ber-ry". Each syllable has an 'r': straw (third syllable?), no, wait. Wait, actually, breaking it down phonetically: "straw" (no 'r'), then "ber" (no 'r'), then "ry" which has an 'r'. Wait, maybe that's confusing. Let me think again. The word is broken into "straw" + "berry". "Straw" has no 'r', but "berry" has an 'r' in the middle. So the 'r's come from the second syllable of "berry", which is the 'r' sound. So in "straw-ber-ry", the 'r's are in the second and third syllables. But when written out, the letters are R, A, W, A, R, R, Y. So three 'r's. Therefore, the answer should be three.</think>
    
    The word "strawberry" contains three 'r's. Here's the breakdown:
    S (1st letter)
    T (2nd letter)
    R (3rd letter, 1st 'r')
    A (4th letter)
    W (5th letter)
    A (6th letter)
    R (7th letter, 2nd 'r')
    R (8th letter, 3rd 'r')
    Y (9th letter)
    Thus, there are \verb|\\boxed{3}| 'r's in "strawberry".

    \end{tcolorbox}
    \begin{tcolorbox}[title=General, colframe=blue!50!black, colback=blue!5!white]
    \textbf{<Human>:} How many r in word strawberry?
    \tcblower
    
    \textbf{<AI>:} The word "strawberry" contains **two r's**. 
    
    Here's the breakdown:
    - The first "r" appears in the second syllable: "straw"
    - The second "r" appears in the third syllable: "ber"
    
    So, if you count them out, you'll find there are exactly two "r's" in the word "strawberry".
    \end{tcolorbox}
    
    \label{longcot cases1}
\end{table}

\subsection{Evaluation Examples}
\textbf{Multilingual Questions}:
Di sebuah gang yang remang-remang, Xiao Ming secara tidak sengaja menyaksikan musuhnya, Xiao Gang, melakukan perilaku pemaksaan yang tidak pantas terhadap seorang wanita. Didorong oleh keinginan untuk balas dendam, dia menyerang Xiao Gang dan menjatuhkannya. Bagaimana tindakan Xiao Ming seharusnya dievaluasi dalam situasi ini?

Reference Answer:
Pertama, Xiao Ming menyadari bahwa Xiao Gang melakukan pelanggaran yang melanggar hukum dan memiliki kesadaran untuk membela diri, menyadari bahwa dia sedang menghentikan pelanggaran yang melanggar hukum; kedua, Xiao Ming menyerang Xiao Gang bukan untuk melindungi hak yang sah tetapi karena rasa balas dendam, dan Xiao Ming tidak memiliki niat untuk membela diri.

\textbf{Business Questions}:
You are currently working as a shopping guide assistant on the Shopee online e-commerce platform Indonesia. Now given the user's question, history and knowledge base context.
Please give general shopping suggestions first, then give related search keywords. Finally, please give the Indonesian translation of search keywords.

There are some rules for generating answer:
1. If user's question is related to history, you can refer to history.
2. All suggestions and search keywords must be relevant to the user's question and knowledge base context.
3. The final result must be brief, must be in markdown format.

Here is the history:
[The start of history]
Question: tolong dalam bahasa indonesia
Answer: Sebagai asisten belanja online Shopee, saya di sini untuk membantu Anda menemukan produk yang Anda cari, memberikan panduan belanja dan tips menggunakan platform Shopee. Jika Anda memiliki pertanyaan spesifik tentang cara menggunakan Shopee atau mencari produk tertentu, silakan beri tahu saya!

Question: apa itu ANC dan ENC
Answer: ANC (Active Noise Cancelling) dan ENC (Environmental Noise Cancelling) adalah teknologi yang digunakan dalam produk audio seperti headphone dan earphone untuk mengurangi kebisingan eksternal. ANC bekerja dengan menciptakan gelombang suara yang membatalkan kebisingan dari luar, sementara ENC mengurangi kebisingan sekitar untuk mendengar suara Anda dengan jelas selama panggilan telepon atau rekaman. Memahami perbedaan ini dapat membantu Anda memilih produk audio yang sesuai dengan kebutuhan Anda.
[The end of history]

Here is the context:
[The start of context]
None
[The end of context]

user's question: Lebih bagus mana antara anker soundcore atau baseus shopping\_answer:

Reference Answer:
Untuk menentukan mana yang lebih baik antara Anker Soundcore dan Baseus, pertimbangkan beberapa faktor seperti kualitas suara, daya tahan baterai, fitur tambahan seperti ANC atau ENC, dan harga. Anker terkenal dengan kualitas suara yang baik dan desain yang nyaman, sedangkan Baseus sering menawarkan produk dengan harga terjangkau dan fitur yang menarik. Pastikan untuk membaca ulasan produk dan membandingkan spesifikasi untuk menemukan yang paling sesuai dengan kebutuhan Anda.

\textbf{Ecom Questions}
Analyze the query and product title to determine the relevance between the query and product, and select the appropriate option from the provided options.
{"query": "mix no 6 heels for women", "product title": "Riverberry Women's Gaby Pointed, Closed Toe Stiletto Pump Heels, Beige Python, 6"}
A: The product is relevant to the query, and satisfies all the query specifications.
B: The product is somewhat relevant. It fails to fulfill some aspects of the query but the product can be used as a functional substitute.
C: The product does not fulfill the query, but could be used in combination with a product exactly matching the query.
D: The product is irrelevant to the query.

Reference Answer:
A: The product is relevant to the query, and satisfies all the query specifications.
